# Supplementary material for: Learning Over Dirty Data with Minimal Repairs
Source: arXiv:2503.13921 source file (2026-03-18)
Supplement: Supplementary file 1 [file supp_archived.tex]

% \section*{\textcolor{red}{TODO}}
% 1. experimental-tables and charts, 2. replace all example with sample, replace all minimal imputation to minimal repair, 3. explain dataset with more details and also the evaluation metrics for linear regression and SVM, 4. Explain in some scenarios MR or AMR don't save (covered in Limitations section but might need some changes), 5. Hyperparameter tuning results with explanation, 6. Link to codebase, 7. Related work



% \section*{Limitations}

% While our work demonstrates both theoretical and practical advantages in learning over incomplete data, we acknowledge two limitations:

% \paragraph{Model Class and Convexity Assumptions.}
% Our proposed minimal repair (MR) algorithms are developed for support vector machines (SVM) and linear regression, while the almost minimal repair (AMR) framework is applicable to a broader class of statistical machine learning models. However, for AMR, we currently provide provable error bounds and efficient approximations only for models with convex loss functions. This stems from our reliance on Step 1 (ST1) in Section~5.1, where we solve a convex optimization problem to find an approximately optimal model $w_k^{\approx}$. Extending AMR to models with non-convex loss functions remains an open challenge due to the difficulty of verifying approximate optimality in such settings. Importantly, this limitation reflects the well-known hardness of non-convex optimization itself—since one cannot generally find globally optimal models for non-convex losses, it is also difficult to guarantee that a repaired model is close to a global optimum.

% \paragraph{Trade-off Between Computation and Imputation Time.}
% As seen in our experiments, the time required to compute MR or AMR can exceed or roughly match the time needed to fully impute the dataset when simple imputation methods (e.g., mean or KNN) are used. This suggests that MR and AMR may not be the preferred choice in scenarios where users already opt for inexpensive imputation strategies. However, for more complex, resource-intensive and often accurate imputation methods—such as diffusion-based models \cite{zheng2022diffusion}—we observe substantial time savings by using MR or AMR to reduce the number of imputations. In practice, users may choose to apply MR or AMR when planning to use high-cost imputation models, and directly pursue full imputation when using simpler methods.


\subsection{Approximating AMR for Deep Neural Networks}

Computing AMR for Deep Neural Networks (DNNs) is challenging as minimizing the suboptimality gap requires global minima for every repair. Recall that an ACM $\mathbf{w}^{\approx}$ satisfies:
\begin{equation}\label{equation:ACM_DNN}
\sup_{\mathbf{X}^r \in \mathbf{X}^R} \left( L(\mathbf{w}^{\approx}, \mathbf{X}^r, \mathbf{y}) - \min_{\mathbf{w} \in \mathcal{W}} L(\mathbf{w}, \mathbf{X}^r, \mathbf{y}) \right) \le e.
\end{equation}
Since flexible DNNs can memorize random data with near-zero loss \cite{zhang2016understanding, cooper2018loss}, we assume $\min_{\mathbf{w} \in \mathcal{W}} L(\mathbf{w}, \mathbf{X}^r, \mathbf{y}) \approx 0$. Thus, checking for an ACM simplifies to ensuring the worst-case loss is bounded.

To make this feasible, we check the condition sample-wise. We verify if the average difference between maximal and minimal repair losses satisfies the threshold $e$:
\begin{equation}\label{equation:ACMcheckdecomposeToSample}
\frac{1}{n} \sum_{\mathbf{x}_i \in MVX} \left( \max_{\mathbf{x}_i^r \in \mathbf{x}_i^R} L(f(\mathbf{x}_i^{r}, \mathbf{w}^{\approx}), y_i) - \min_{\mathbf{x}_i^r \in \mathbf{x}_i^R} L(f(\mathbf{x}_i^{r}, \mathbf{w}^{\approx}), y_i) \right) \leq e
\end{equation}
For networks with monotonic activations (e.g., ReLU), extrema occur at missing value boundaries (edge repairs), significantly reducing cost.

When the ACM condition is violated, AMR is the smallest subset restoring it. Intuitively, we impute samples contributing most to the loss difference in Eq. \ref{equation:ACMcheckdecomposeToSample}. Since this ranking is model-dependent, Algorithm \ref{alg:DNNAMR} collaboratively learns the DNN and identifies AMR via SGD.

\begin{algorithm}[!htbp]
\caption{Approximating AMR for Neural Networks}\label{alg:DNNAMR}
\begin{algorithmic}
\STATE $S_{AMR} \gets [\quad]$
\STATE $\mathbf{X}^{curr} \gets \text{random repair of } \mathbf{X}$; $\mathbf{w}^{curr} \gets \text{random initialization}$
\STATE $maxL, minL, samplesTopK \gets checkACM(\mathbf{w}^{curr}, \mathbf{X}^{curr})$
\WHILE{$maxL - minL > e$}
    \IF{$maxL > e$ \textbf{AND} $minL \leq e$}
        \STATE $\mathbf{X}^{curr} \gets impute(\mathbf{X}^{curr}, samplesTopK)$
        \STATE $S_{AMR} \gets S_{AMR}.add(samplesTopK)$
    \ENDIF
    \STATE $\mathbf{w}^{curr} \gets SGDEpoch(\mathbf{w}^{curr}, \mathbf{X}^{curr})$
    \STATE Update $maxL, minL, samplesTopK$
\ENDWHILE
\STATE \textbf{return} $S_{AMR}$
\end{algorithmic}
\end{algorithm}

The algorithm iteratively identifies $k$ samples to restore the ACM condition. Crucially, we only impute when the model is ``approximately optimal'' for some repairs ($minL \le e < maxL$). If both losses exceed $e$, we prioritize training ($SGDEpoch$) to ensure selection reflects true sample importance. $S_{AMR}$ is the union of imputed samples.
